# Supplementary material for: Centralized Matching with Incomplete Information
Source: arXiv:2107.04098 ancillary file (2021-07-08)
Supplement: Supplementary file 1 [file IncompleteInfoMatchingAppendix.pdf]

# Online Appendix for "Centralized Matching with Incomplete Information"

by Marcelo Ariel Fernandez, Kirill Rudov, and Leeat Yariv

July 6, 2021

**Abstract**

This Online Appendix contains the following items. First, in Appendix A, we provide additional examples that the main text refers to. Second, in Appendix B, we provide all proofs omitted from the main text. Third, Appendix C describes extensions of our positive results. Finally, in Appendix D, we provide fragility results for a large class of stable mechanisms.

## A. Additional Examples

**Example 1** (generalized motivating example). *The example has the following features:*

1. *there is no uncertainty on the unique stable matching;*
2. *there is a BNE that supports unstable outcomes in both states;*
3. *any BNE outcome can be supported by weakly undominated strategies that induce a unique stable matching (with respect to reported preferences) in each state;*
4. *all unstable BNE outcomes ex-ante Pareto dominate the stable one for workers;*
5. *the set of matched workers varies across equilibrium outcomes. Furthermore, workers disagree on which is preferred.*

Consider an economy with three firms: $f_1$, $f_2$, and $f_3$ and three workers: $w_1$, $w_2$, and $w_3$. There are two states of the world: $\Theta = \{1, 2\}$, distributed according to non-degenerate binary distribution $\Psi$. For state $\theta \in \Theta$, the preferences are given by $U(\theta)$ as follows:

$U(1)$

| | | | |
|---|---|---|---|
| | $\mathbf{3, 2}$ | $1, 2.5/\rho$ | $2, 2$ |
| $\boldsymbol{\mu}$ | $2, 2.5/\rho$ | $\mathbf{3, 2}$ | $1, 2.5/\rho$ |
| | $1, 1$ | $2, 1$ | $\mathbf{3, 1}$ |

$U(2)$

| | | |
|---|---|---|
| $\mathbf{3, 2}$ | $1, 2.5/\rho$ | $2, 2$ |
| $1, 2.5/\rho$ | $\mathbf{3, 2}$ | $2, 2.5/\rho$ |
| $1, 1$ | $2, 1$ | $\mathbf{3, 1}$ |

where $\rho \equiv \min(\Psi(1), 1 - \Psi(1))$. This example generalizes the motivating example corresponding to equally likely states, i.e. $\Psi(1) = 1/2$.

In both states, there is a unique complete-information stable matching $\mu$, $\mu(f_i) = w_i$ for $i \in \{1, 2, 3\}$, highlighted in bold. As in the motivating example, despite information being incomplete, there is no uncertainty regarding the stable matching. The only difference

between the two states appears in $f_2$'s preferences—she ranks $w_1$ and $w_3$ differently across the states.

As mentioned in the main text, the complete-information stable matching in each state is supported as an equilibrium outcome of the game induced by the firm-proposing DA. We now show this outcome is not unique. In fact, there are *three other equilibrium outcomes*, all of which are *unstable*. Furthermore, all these equilibrium outcomes can be supported by weakly undominated strategies.

*First,* consider the equilibrium outcome denoted by $\lambda_1$, with $\lambda_1(1), \lambda_1(2) \neq \mu$,

| | $U(1)$ | | | $U(2)$ | | |
|---|---|---|---|---|---|---|
| | $\mathbf{3, 2}$ | $1, 2.5/\rho$ | $2, 2$ | $\mathbf{3, 2}$ | $1, 2.5/\rho$ | $2, 2$ |
| $\lambda_1$ | $2, 2.5/\rho$ | $\mathbf{3, 2}$ | $1, 2.5/\rho$ | $1, 2.5/\rho$ | $\mathbf{3, 2}$ | $2, 2.5/\rho$ |
| | $1, 1$ | $2, 1$ | $\mathbf{3, 1}$ | $1, 1$ | $2, 1$ | $\mathbf{3, 1}$ |

supported by the following profile of workers' weakly undominated strategies:

- worker $w_1$ drops $f_1$;
- worker $w_3$ drops $f_1$;
- worker $w_2$ reports truthfully.

We can also reformulate this profile in an equivalent matrix notation:

$$\begin{pmatrix} \emptyset & 3 & \emptyset \\ 2 & 2 & 2 \\ 1 & 1 & 1 \end{pmatrix},$$

where the strategically reported preferences of worker $w_j$, $j \in \{1, 2, 3\}$, over firms $f_i$, $i \in \{1, 2, 3\}$, correspond to column $j$ with $\emptyset$ denoting unacceptable firms (this convention

economizes on notation and will be followed throughout this Online Appendix). This profile generates the stable matchings—for the reported preferences—denoted $\lambda_1(1)$ and $\lambda_1(2)$ in states 1 (left) and 2 (right), respectively. Also, these matchings are unique stable for the reported preferences.

The proposed profile indeed constitutes an equilibrium:

- Worker $w_1$ cannot get his most preferred firm, $f_2$, in state 2. In order to get his second most preferred firm, $f_1$, in state 2, $w_1$ needs to report $f_1$ to be more preferable than $f_3$. However, such deviation precludes him from getting his most preferable $f_2$ in state 1. The corresponding utility from $f_2$ is sufficiently high, so that $w_1$ has no incentives to deviate.
- Similarly, $w_3$ has no incentives to deviate.
- Worker $w_2$ has no incentives to deviate from his truthful strategy since the induced matchings are unique for reported preferences.

In addition, three other equilibrium profiles induce $\lambda_1$:

$$\begin{pmatrix} \emptyset & 2 & \emptyset \\ 2 & 1 & 2 \\ 1 & \emptyset & 1 \end{pmatrix}, \quad \text{or} \quad \begin{pmatrix} \emptyset & 2 & 1 \\ 2 & 1 & 3 \\ 1 & \emptyset & 2 \end{pmatrix}, \quad \text{or} \quad \begin{pmatrix} \emptyset & 3 & 1 \\ 2 & 2 & 3 \\ 1 & 1 & 2 \end{pmatrix}.$$

*Second,* there is an equilibrium outcome $\lambda_2$, with $\lambda_2(1), \lambda_2(2) \neq \mu$,

$\lambda_2$

$U(1)$

| | | |
|---|---|---|
| $\mathbf{3, 2}$ | $1, 2.5/\rho$ | $2, 2$ |
| $2, 2.5/\rho$ | $\mathbf{3, 2}$ | $1, 2.5/\rho$ |
| $1, 1$ | $2, 1$ | $\mathbf{3, 1}$ |

$U(2)$

| | | |
|---|---|---|
| $\mathbf{3, 2}$ | $1, 2.5/\rho$ | $2, 2$ |
| $1, 2.5/\rho$ | $\mathbf{3, 2}$ | $2, 2.5/\rho$ |
| $1, 1$ | $2, 1$ | $\mathbf{3, 1}$ |

supported by the following profile of weakly undominated strategies for workers:

$$\begin{pmatrix} \emptyset & 3 & 2 \\ 2 & 1 & 3 \\ 1 & 2 & 1 \end{pmatrix}.$$

There are no other equilibrium profiles—even if we allow for weakly dominated strategies—supporting $\lambda_2$.

*Third,* there is one more equilibrium outcome $\lambda_3$, with $\lambda_3(1), \lambda_3(2) \neq \mu$,

$\lambda_3$

$U(1)$

| | | |
|---|---|---|
| $\mathbf{3, 2}$ | $1, 2.5/\rho$ | $2, 2$ |
| $2, 2.5/\rho$ | $\mathbf{3, 2}$ | $1, 2.5/\rho$ |
| $1, 1$ | $2, 1$ | $\mathbf{3, 1}$ |

$U(2)$

| | | |
|---|---|---|
| $\mathbf{3, 2}$ | $1, 2.5/\rho$ | $2, 2$ |
| $1, 2.5/\rho$ | $\mathbf{3, 2}$ | $2, 2.5/\rho$ |
| $1, 1$ | $2, 1$ | $\mathbf{3, 1}$ |

which can be supported by either of the following two profiles:

$$\begin{pmatrix} 1 & 3 & \emptyset \\ 3 & 2 & 1 \\ 2 & 1 & \emptyset \end{pmatrix} \quad \text{or} \quad \begin{pmatrix} 1 & 2 & \emptyset \\ 3 & 1 & 1 \\ 2 & \emptyset & \emptyset \end{pmatrix}.$$

Note that $w_3$ is unmatched in state 1 under $\lambda_3$, i.e. the set of matched workers varies across equilibrium outcomes. Also, worker $w_2$ prefers $\lambda_1$, while worker $w_3$ prefers $\lambda_2$. Thus, workers disagree on which equilibrium outcome is preferred.[1] It is straightforward to check all other stated features of the example. △

**Example 2** (alternative fragility example)**.** *For the proof of Proposition 3, we need an additional fragility example that is similar to Example 1 above and has the following features:*

[1] In fact, firms also disagree on their preferred equilibrium outcome. Indeed, firm $f_3$ prefers $\lambda_1$ to $\lambda_2$ while firm $f_1$ prefers $\lambda_2$ to $\lambda_1$.

1. *there is a BNE that supports unstable outcomes in both states;*
2. *any BNE outcome can be supported by weakly undominated strategies that induce a unique stable matching (with respect to reported preferences) in each state;*
3. *the set of matched workers varies across equilibrium outcomes. Furthermore, workers disagree on which is preferred.*

Consider, as before, an economy with three firms and three workers, with two states of the world: $\Theta = \{1, 2\}$, distributed according to a non-degenerate binary distribution $\Psi$. Preferences are given by $U(\theta)$ as follows:

$U(1)$

| | | | |
|---|---|---|---|
| | $3, 2$ | $\boldsymbol{2, 2.5/\rho}$ | $1, 1$ |
| $\boldsymbol{\mu}$ | $1, 1$ | $3, 2$ | $\boldsymbol{2, 2}$ |
| | $\boldsymbol{2, 2.5/\rho}$ | $3, 1$ | $1, 2.5/\rho$ |

$U(2)$

| | | |
|---|---|---|
| $\boldsymbol{3, 2}$ | $2, 2.5/\rho$ | $1, 1$ |
| $1, 1$ | $\boldsymbol{3, 2}$ | $2, 2$ |
| $1, 2.5/\rho$ | $3, 1$ | $\boldsymbol{2, 2.5/\rho}$ |

where $\rho \equiv \min(\Psi(1), 1 - \Psi(1))$.

In each state, there is a (state-specific) unique complete-information stable matching highlighted in bold in the payoff matrices above, so that $\mu(1)(f_1) = w_2$, $\mu(1)(f_2) = w_3$, and $\mu(1)(f_3) = w_1$, and $\mu(2)(f_i) = w_i$ for $i \in \{1, 2, 3\}$. The only payoff uncertainty is how firm 3 ranks worker 1 and worker 3.

As before, the complete-information stable matching in each state is an equilibrium outcome of this game. Indeed, workers reporting their preferences truthfully constitutes an equilibrium. However, we will now show that it is not unique. In fact, there are *two other equilibrium outcomes*, both of which are *unstable*. Furthermore, these equilibrium outcomes can be supported by weakly undominated strategies.

*First,* there is an equilibrium outcome denoted by $\lambda_1$, with $\lambda_1(2) \neq \mu(2)$, but $\lambda_1(1) = \mu(1)$,

| | $U(1)$ | | | $U(2)$ | | |
|---|---|---|---|---|---|---|
| | $3, 2$ | $\boldsymbol{2, 2.5/\rho}$ | $1, 1$ | $\boldsymbol{3, 2}$ | $2, 2.5/\rho$ | $1, 1$ |
| $\lambda_1$ | $1, 1$ | $3, 2$ | $\boldsymbol{2, 2}$ | $1, 1$ | $\boldsymbol{3, 2}$ | $2, 2$ |
| | $\boldsymbol{2, 2.5/\rho}$ | $3, 1$ | $1, 2.5/\rho$ | $1, 2.5/\rho$ | $3, 1$ | $\boldsymbol{2, 2.5/\rho}$ |

supported by either of the following eight profiles:

$$\begin{pmatrix} \emptyset & 2 & 1 \\ 1 & \emptyset & 2 \\ 2 & 1 & 3 \end{pmatrix}, \quad \text{or} \quad \begin{pmatrix} \emptyset & 2 & \emptyset \\ 1 & \emptyset & 1 \\ 2 & 1 & 2 \end{pmatrix}, \quad \text{or} \quad \begin{pmatrix} \emptyset & 2 & 2 \\ 1 & \emptyset & 1 \\ 2 & 1 & 3 \end{pmatrix}, \quad \text{or} \quad \begin{pmatrix} \emptyset & 3 & \emptyset \\ 1 & 1 & 1 \\ 2 & 2 & 2 \end{pmatrix},$$

$$\text{or} \quad \begin{pmatrix} \emptyset & 3 & 2 \\ 1 & 1 & 1 \\ 2 & 2 & 3 \end{pmatrix}, \quad \text{or} \begin{pmatrix} \emptyset & 3 & 1 \\ 1 & 1 & 2 \\ 2 & 2 & 3 \end{pmatrix}, \quad \text{or} \quad \begin{pmatrix} \emptyset & 2 & 3 \\ 1 & \emptyset & 1 \\ 2 & 1 & 2 \end{pmatrix}, \quad \text{or} \quad \begin{pmatrix} \emptyset & 3 & 3 \\ 1 & 1 & 1 \\ 2 & 2 & 2 \end{pmatrix},$$

with, say, the first of them being in workers' weakly undominated strategies.

*Second,* there is another equilibrium outcome $\lambda_2$, with $\lambda_2(1) \neq \mu(1)$ and $\lambda_2(2) \neq \mu(2)$,

| | $U(1)$ | | | $U(2)$ | | |
|---|---|---|---|---|---|---|
| | $3, 2$ | $\boldsymbol{2, 2.5/\rho}$ | $1, 1$ | $\boldsymbol{3, 2}$ | $2, 2.5/\rho$ | $1, 1$ |
| $\lambda_2$ | $1, 1$ | $3, 2$ | $\boldsymbol{2, 2}$ | $1, 1$ | $\boldsymbol{3, 2}$ | $2, 2$ |
| | $\boldsymbol{2, 2.5/\rho}$ | $3, 1$ | $1, 2.5/\rho$ | $1, 2.5/\rho$ | $3, 1$ | $\boldsymbol{2, 2.5/\rho}$ |

supported by any of the following six profiles:

$$\begin{pmatrix} 1 & 3 & 1 \\ 2 & 1 & \emptyset \\ 3 & 2 & 2 \end{pmatrix}, \quad \text{or} \quad \begin{pmatrix} 1 & 2 & \emptyset \\ 2 & \emptyset & \emptyset \\ 3 & 1 & 1 \end{pmatrix}, \quad \text{or} \quad \begin{pmatrix} 1 & 2 & 1 \\ 2 & \emptyset & \emptyset \\ 3 & 1 & 2 \end{pmatrix}, \quad \text{or} \quad \begin{pmatrix} 1 & 3 & \emptyset \\ 2 & 1 & \emptyset \\ 3 & 2 & 1 \end{pmatrix},$$

$$\text{or} \quad \begin{pmatrix} 1 & 2 & 2 \\ 2 & \emptyset & \emptyset \\ 3 & 1 & 1 \end{pmatrix}, \quad \text{or} \quad \begin{pmatrix} 1 & 3 & 2 \\ 2 & 1 & \emptyset \\ 3 & 2 & 1 \end{pmatrix},$$

where again, say, the first profile involves weakly undominated strategies for workers.

It is straightforward to verify all stated features for this example. △

**Example 3** (economy with assortative preferences for firms violating the SPC*)**.** *The example has the following features:*

1. *firms have (state-dependent) assortative preferences in each state;*
2. *the SPC* is violated.*

Consider, again, an economy with three firms, three workers, and two states of the world:

$U(1)$

| | | |
|---|---|---|
| **3, 3** | 2, 3 | 1, 1 |
| 3, 2 | **2, 2** | 1, 2 |
| 3, 1 | 2, 1 | **1, 3** |

$U(2)$

| | | |
|---|---|---|
| 1, 3 | **2, 3** | 3, 1 |
| **1, 2** | 2, 2 | 3, 2 |
| 1, 1 | 2, 1 | **3, 3** |

This economy satisfies the SPC with the corresponding state-dependent orderings being

defined uniquely, so that the respective sequential top-top match pairs are:

$$\theta = 1 : (f_1, w_1), (f_2, w_2), (f_3, w_3);$$

$$\theta = 2 : (f_3, w_3), (f_1, w_2), (f_2, w_1),$$

However, it does not satisfy the SPC*. Indeed, in state 1, worker $w_2$ of order 2 prefers firm $f_1$ over his stable partner $f_2$, but this "demanded" firm $f_1$ has order 2 (not 1, as required by the SPC*) in state 2. △

**Example 4** (economy with a preference cycle satisfying the SPC*)**.** *The example has the following features:*

1. *the SPC* is satisfied;*

2. *there is a preference cycle.*

Consider an economy with three firms, three workers, and two states. For state 1, there is a cycle in the preferences given by $U(1)$ as follows:

$U(1)$

| | | |
|---|---|---|
| **3, 3** | 1, 3 | 2, 2 |
| 3, 1 | **2, 2** | 1, 3 |
| 2, 2 | 1, 1 | **3, 1** |

This market satisfies the SPC with the corresponding firms' and workers' orderings being defined uniquely, so that the respective sequential top-top match pairs are

$$\theta = 1 : (f_1, w_1), (f_2, w_2), (f_3, w_3).$$

What restrictions does the condition of the SPC* impose on $U(2)$? In state 1, worker $w_2$ of order 2 prefers firm $f_1$ over his stable partner $f_2$. Also, worker $w_3$ of order 3 prefers both

$f_1$ and $f_2$ over his stable partner $f_3$. Therefore, by the SPC*, in state 2, firm $f_1$ must have order 1 and firm $f_2$ must have order 2.

The SPC* is satisfied, say, if we consider the following $U(2)$:

$U(2)$

| | | |
|---|---|---|
| $1,3$ | $\mathbf{3,3}$ | $2,2$ |
| $1,1$ | $3,2$ | $\mathbf{2,3}$ |
| $\mathbf{2,2}$ | $1,1$ | $3,1$ |

It satisfies the SPC for

$$\theta = 2 : (f_1, w_2), (f_2, w_3), (f_3, w_1). \qquad \triangle$$

**Example 5** (economy satisfying the SPC* and having no preference cycles with non-assortative preferences for workers)**.** *The example has the following features:*

1. *the SPC* is satisfied;*
2. *there are no preference cycles;*
3. *workers' preferences are not assortative.*

Consider an economy with four firms, four workers, and two states:

$U(1)$

| | | | |
|---|---|---|---|
| $\mathbf{4,4}$ | $3,4$ | $2,2$ | $1,1$ |
| $2,1$ | $\mathbf{4,3}$ | $3,3$ | $1,2$ |
| $1,2$ | $4,2$ | $\mathbf{3,4}$ | $2,4$ |
| $3,3$ | $2,1$ | $1,1$ | $\mathbf{4,3}$ |

$U(2)$

| | | | |
|---|---|---|---|
| $3,4$ | $\mathbf{4,4}$ | $2,2$ | $1,1$ |
| $3,1$ | $4,3$ | $\mathbf{2,3}$ | $1,2$ |
| $2,2$ | $4,2$ | $1,4$ | $\mathbf{3,4}$ |
| $\mathbf{3,3}$ | $1,1$ | $2,1$ | $4,3$ |

First, there are no preference cycles since for each state $\theta$, *ordinal* preferences corresponding to $U(\theta)$ can be described by using one matrix $P(\theta)$, also called an *ordinal potential*, see Ferdowsian, Niederle, and Yariv (2021):

$P(1)$

| | | | |
|---|---|---|---|
| **16** | 15 | 4 | 1 |
| 6 | **14** | 11 | 2 |
| 7 | 13 | **12** | 10 |
| 8 | 5 | 3 | **9** |

$P(2)$

| | | | |
|---|---|---|---|
| 15 | **16** | 5 | 2 |
| 8 | 14 | **6** | 3 |
| 9 | 13 | 7 | **12** |
| **10** | 1 | 4 | 11 |

Second, this economy satisfies the SPC*. Indeed, the SPC holds with the respective sequential top-top match pairs:

$$\theta = 1 : (f_1, w_1), (f_2, w_2), (f_3, w_3), (f_4, w_4);$$

$$\theta = 2 : (f_1, w_2), (f_3, w_4), (f_4, w_1), (f_2, w_3).$$

What restrictions does the condition of the SPC* impose on $U(1)$ and $U(2)$? In state 1, worker $w_2$ of order 2 prefers firm $f_1$ over his stable partner $f_1$. Also, worker $w_4$ of order 4 prefers $f_3$ over his stable partner $f_4$. Therefore, by the SPC*, in state 2, firm $f_1$ must have order 1 and firm $f_3$ must have order at most 3.

Similarly, in state 2, worker $w_1$ of order 3 prefers firm $f_1$ over his stable partner $f_4$. Furthermore, worker $w_3$ of order 4 prefers $f_3$ over his stable partner $f_2$. Therefore, by the SPC*, in state 1, firm $f_1$ must have order at most 2 and firm $f_3$ must have order at most 3.

To conclude, all restrictions imposed by the SPC* are indeed satisfied and, in either state, workers' preferences are not assortative, as desired. △

**Example 6** (instability with the SPC)**.** *The example has the following features:*

1. *the SPC is satisfied;*

2. *the SPC* is violated;*

*3. there is a BNE in weakly undominated strategies that supports unstable outcomes in both states.*

Consider an economy with five firms, five workers, and two equally-likely states:

$U(1)$

| | | | | |
|---|---|---|---|---|
| **5, 5** | 3, 6 | 2, 2 | 4, 4 | 1, 3 |
| 5, 3 | **4, 4** | 3, 4 | 2, 5 | 1, 2 |
| 5, 2 | 4, 3 | **1, 3** | 2, 2 | 3, 1 |
| 1, 4 | 2, 2 | 4, 6 | **5, 3** | 3, 5 |
| 2, 1 | 1, 1 | 3, 1 | 4, 1 | **5, 4** |

$\boldsymbol{\mu}$

$U(2)$

| | | | | |
|---|---|---|---|---|
| 2, 5 | 4, 6 | 3, 2 | **5, 4** | 1, 3 |
| 2, 3 | 4, 4 | **5, 4** | 3, 5 | 1, 2 |
| 1, 2 | **5, 3** | 4, 3 | 2, 2 | 3, 1 |
| 1, 4 | 2, 2 | 3, 6 | 4, 3 | **5, 5** |
| **2, 1** | 1, 1 | 3, 1 | 4, 1 | 5, 4 |

In each state, there is a (state-specific) unique complete-information stable matching highlighted in bold in the payoff matrices above, so that $\mu(1)(f_i) = w_i$ for any $i \in [5]$, and $\mu(2)(f_1) = w_4$, $\mu(2)(f_2) = w_3$, $\mu(2)(f_3) = w_2$, $\mu(2)(f_4) = w_5$, and $\mu(2)(f_5) = w_1$.

Although this economy satisfies the SPC, say, with the corresponding sequential top-top match pairs:

$$\theta = 1 : (f_1, w_1), (f_2, w_2), (f_4, w_4), (f_5, w_5), (f_3, w_3);$$

$$\theta = 2 : (f_4, w_5), (f_2, w_3), (f_1, w_4), (f_3, w_2), (f_5, w_1),$$

it does not satisfy the restriction of the SPC*. Indeed, in state 1, $(f_2, w_2)$ must have order 2, irrespective of the employed orderings. In this pair, worker $w_2$ prefers firm $f_1$ over his stable partner $f_2$, but this firm $f_1$ cannot have order 1 in state 2, as required by the SPC*. That is, the SPC* is violated.

The equilibrium outcome denoted by $\lambda$, with $\lambda(1) \neq \mu(1)$ and $\lambda(2) \neq \mu(2)$,

$\lambda$

$U(1)$

| | | | | |
|---|---|---|---|---|
| $\mathbf{5, 5}$ | $3, 6$ | $2, 2$ | $4, 4$ | $1, 3$ |
| $5, 3$ | $\mathbf{4, 4}$ | $3, 4$ | $2, 5$ | $1, 2$ |
| $5, 2$ | $4, 3$ | $\mathbf{1, 3}$ | $2, 2$ | $3, 1$ |
| $1, 4$ | $2, 2$ | $4, 6$ | $\mathbf{5, 3}$ | $3, 5$ |
| $2, 1$ | $1, 1$ | $3, 1$ | $4, 1$ | $\mathbf{5, 4}$ |

$U(2)$

| | | | | |
|---|---|---|---|---|
| $2, 5$ | $4, 6$ | $3, 2$ | $\mathbf{5, 4}$ | $1, 3$ |
| $2, 3$ | $4, 4$ | $\mathbf{5, 4}$ | $3, 5$ | $1, 2$ |
| $1, 2$ | $\mathbf{5, 3}$ | $4, 3$ | $2, 2$ | $3, 1$ |
| $1, 4$ | $2, 2$ | $3, 6$ | $4, 3$ | $\mathbf{5, 5}$ |
| $\mathbf{2, 1}$ | $1, 1$ | $3, 1$ | $4, 1$ | $5, 4$ |

is supported by the following profile of workers' weakly undominated strategies:

- $w_2$ drops $f_2$;
- $w_3$ drops $f_2$;
- everyone else reports truthfully.

This profile generates the stable matchings—for the reported preferences—$\lambda(1)$ and $\lambda(2)$ in states 1 (left) and 2 (right), respectively. Also, these matchings are unique stable for the reported preferences.

The proposed profile indeed constitutes an equilibrium:

- Worker $w_2$ cannot get his most preferred $f_1$ in state 1. In order to get his second most preferred $f_2$ in state 1, $w_2$ needs to report $f_2$ to be preferable to $f_3$. However, such a deviation precludes him from getting his most preferred $f_1$ in state 2. The corresponding utility from $f_1$ is sufficiently high, so that $w_2$ has no incentives to deviate.
- Similarly, worker $w_3$ has no incentives to deviate.
- Other workers have no incentives to deviate from their truthful strategies since the induced matchings are unique for the reported preferences. $\triangle$

**Example 7** (instability with no preference cycles in one state)**.** *The example has the following features:*

1. *there are no preference cycles in one state;*

2. *there is a BNE in weakly undominated strategies that supports unstable outcome in one state.*

Consider an economy with four firms, four workers, and two equally-likely states:

$\boldsymbol{\mu}$

$U(1)$

| | | | |
|---|---|---|---|
| **4, 4** | 3, 5 | 2, 1 | 1, 1 |
| 2, 2 | **4, 3** | 3, 4 | 1, 2 |
| 2, 3 | 3, 2 | **4, 3** | 1, 3 |
| 2, 1 | 1, 1 | 4, 2 | **3, 4** |

$U(2)$

| | | | |
|---|---|---|---|
| 1, 4 | **3, 5** | 2, 1 | 4, 1 |
| 2, 2 | 4, 3 | **3, 4** | 1, 2 |
| **2, 3** | 3, 2 | 4, 3 | 1, 3 |
| 2, 1 | 1, 1 | 4, 2 | **3, 4** |

In each state, there is a (state-specific) unique complete-information stable matching highlighted in bold in the payoff matrices above, so that $\mu(1)(f_i) = w_i$ for any $i \in [4]$, and $\mu(2)(f_1) = w_2$, $\mu(2)(f_2) = w_3$, $\mu(2)(f_3) = w_1$, and $\mu(2)(f_4) = w_4$. The only payoff uncertainty is whether $w_1$ or $w_4$ is the most (least) desirable for firm $f_1$.

There are no preference cycles in state 1 since *ordinal* preferences corresponding to $U(1)$ can be described by using the following *ordinal potential* matrix $P(1)$:

$P(1)$

| | | | |
|---|---|---|---|
| **16** | 15 | 4 | 1 |
| 7 | **14** | 13 | 2 |
| 8 | 11 | **12** | 3 |
| 6 | 5 | 10 | **9** |

The equilibrium outcome denoted by $\lambda$, with $\lambda(1) \neq \mu(1)$ and $\lambda(2) = \mu(2)$,

$U(1)$

| | | | |
|---|---|---|---|
| $\mathbf{4,4}$ | $3,5$ | $2,1$ | $1,1$ |
| $2,2$ | $\mathbf{4,3}$ | $3,4$ | $1,2$ |
| $2,3$ | $3,2$ | $\mathbf{4,3}$ | $1,3$ |
| $2,1$ | $1,1$ | $4,2$ | $\mathbf{3,4}$ |

$U(2)$

| | | | |
|---|---|---|---|
| $1,4$ | $\mathbf{3,5}$ | $2,1$ | $4,1$ |
| $2,2$ | $4,3$ | $\mathbf{3,4}$ | $1,2$ |
| $\mathbf{2,3}$ | $3,2$ | $4,3$ | $1,3$ |
| $2,1$ | $1,1$ | $4,2$ | $\mathbf{3,4}$ |

$\lambda$

is supported by the following profile of workers' weakly undominated strategies:

- $w_2$ permutes $f_2$ and $f_3$ and reports $f_1 \succ f_3 \succ f_2 \succ f_4$;
- $w_3$ permutes $f_3$ and $f_4$ and reports $f_2 \succ f_4 \succ f_3 \succ f_1$;
- everyone else reports truthfully.

This profile generates the stable matchings—for the reported preferences—$\lambda(1)$ and $\lambda(2)$ in states 1 (left) and 2 (right), respectively. Also, these matchings are unique stable for reported preferences.

The proposed profile indeed constitutes an equilibrium:

- Worker $w_2$ cannot get his most preferred $f_1$ in state 1. In order to get his second most preferred $f_2$ in state 1, $w_2$ needs to report $f_2$ as preferable to $f_3$. However, such a deviation precludes him from getting his most preferred $f_1$ in state 2. The corresponding utility from $f_1$ is sufficiently high, so that $w_2$ has no incentives to deviate.
- Worker $w_3$ gets his favorite firm $f_2$ in both states and has no incentives to deviate.
- Other workers have no incentives to deviate from their truthful strategies since the induced matchings are unique for the reported preferences. $\triangle$

**Example 8** (instability with firms' assortative preferences in one state)**.** *The example has the following features:*

1. *firms have assortative preferences in one state;*

2. *there is a BNE in weakly undominated strategies that supports unstable outcome in one state.*

Consider an economy with three firms, three workers, and two equally-likely states:

| | $U(1)$ | | | $U(2)$ | | |
|---|---|---|---|---|---|---|
| | **1, 2** | 3, 1 | 2, 1 | 2, 2 | **1, 1** | 3, 1 |
| $\boldsymbol{\mu}$ | 1, 1 | **3, 4** | 2, 4 | 3, 1 | 1, 4 | **2, 4** |
| | 1, 4 | 3, 2 | **2, 2** | **2, 4** | 1, 2 | 3, 2 |

In each state, there is a (state-specific) unique complete-information stable matching highlighted in bold in the payoff matrices above, so that $\mu(1)(f_i) = w_i$ for any $i \in [3]$, and $\mu(2)(f_1) = w_2$, $\mu(2)(f_2) = w_3$, and $\mu(2)(f_3) = w_1$.

In addition, firms have assortative preferences in state 1.

The equilibrium outcome denoted by $\lambda$, with $\lambda(1) \neq \mu(1)$ and $\lambda(2) = \mu(2)$,

| | $U(1)$ | | | $U(2)$ | | |
|---|---|---|---|---|---|---|
| | **1, 2** | 3, 1 | 2, 1 | 2, 2 | **1, 1** | 3, 1 |
| $\lambda$ | 1, 1 | **3, 4** | 2, 4 | 3, 1 | 1, 4 | **2, 4** |
| | 1, 4 | 3, 2 | **2, 2** | **2, 4** | 1, 2 | 3, 2 |

is supported by the following profile of workers' weakly undominated strategies:

- $w_1$ drops $f_1$;
- $w_3$ drops $f_3$;
- worker $w_2$ reports truthfully.

This profile generates the stable matchings—for the reported preferences—$\lambda(1)$ and $\lambda(2)$ in states 1 (left) and 2 (right), respectively. Also, these matchings are unique stable for the reported preferences.

The proposed profile indeed constitutes an equilibrium:

- Worker $w_1$ has no incentives to deviate.

- Worker $w_3$ cannot get his most preferred $f_2$ in state 1. In order to get his second most preferred $f_3$ in state 1, $w_3$ needs to report $f_3$ as preferable to $f_1$. However, such a deviation precludes him from getting his most preferred $f_2$ in state 2. The corresponding utility from $f_2$ is sufficiently high, so that $w_3$ has no incentives to deviate.

- Worker $w_2$ has no incentives to deviate from his truthful strategy since the induced matchings are unique for the reported preferences. $\triangle$

**Example 9** (benefits of increased competition)**.** In complete-information matching markets, when focusing on stable outcomes, the addition of competition on one side of the market cannot improve the matches of any participant on that market side and cannot harm the matches of participants on the other market side, see Roth and Sotomayor (1992). Since firm-proposing DA equilibrium outcomes coincide with the stable outcomes, the same implications of increased competition hold. The following example illustrates that this need not be the case with incomplete information. In particular, we show that the addition of one worker may be beneficial for some workers in the economy.

*The example has the following features:*

1. *in the original economy, there is a unique (stable) BNE outcome;*

2. *when augmented with one additional worker, it has an (unstable) BNE outcome supported by weakly undominated strategies that improves the outcome of one of the original workers in the original BNE outcome.*

Consider an *original* economy with three firms and three workers. There are three equally-likely states of the world: $\Theta = \{1, 2, 3\}$. For state $\theta \in \Theta$, the preferences are given by $U(\theta)$ as follows:

$U(1)$

| | | |
|---|---|---|
| $2,5$ | $4,1$ | $\mathbf{3,2}$ |
| $\mathbf{4,2}$ | $3,5$ | $2,5$ |
| $3,1$ | $\mathbf{4,2}$ | $1,1$ |

$U(2)$

| | | |
|---|---|---|
| $\mathbf{3,5}$ | $2,1$ | $1,2$ |
| $3,2$ | $1,5$ | $\mathbf{2,5}$ |
| $4,1$ | $\mathbf{3,2}$ | $2,1$ |

$U(3)$

| | | |
|---|---|---|
| $\mathbf{2,5}$ | $1,1$ | $4,2$ |
| $2,2$ | $1,5$ | $\mathbf{3,5}$ |
| $3,1$ | $\mathbf{1,2}$ | $2,1$ |

In each state, there is a (state-specific) unique complete-information stable matching highlighted in bold in the payoff matrices above, so that (1) $\mu(1)(f_1) = w_3$, $\mu(1)(f_2) = w_1$, $\mu(1)(f_3) = w_2$, (2) $\mu(2)(f_1) = w_1$, $\mu(2)(f_2) = w_3$, $\mu(2)(f_3) = w_2$, and (3) $\mu(3) = \mu(2)$.

This economy admits a unique BNE outcome corresponding to the unique (complete-information) stable outcome in each state. Indeed, in any equilibrium profile,

- Worker $w_1$ must report firm $f_1$ as acceptable and rank her above both $f_2$ and $f_3$. If not, worker $w_1$ could profitably deviate by shifting $f_1$ to the top of his ranking to strictly benefit in state 2 without losing in states 1 and 3.

- Also, worker $w_3$ must report $f_2$ as acceptable and rank her above both $f_1$ and $f_3$. If not, worker $w_3$ could profitably deviate by shifting $f_2$ to the top of his ranking to strictly benefit in state 3 without losing in states 1 and 2.

  Therefore, in states 2 and 3, $w_1$ and $w_3$ must be matched to $f_1$ and $f_2$, respectively.

- Worker $w_1$ is not matched with $f_1$ in state 1. If he is, then $w_2$ gets his favorite $f_2$ (otherwise, he could deviate by shifting $f_2$ to the top) and hence $w_3$ could get $f_1$ (by moving $f_1$ just below $f_2$), in contradiction. Since $w_1$ is not matched with $f_1$ in state 1, he must report $f_2$ as acceptable.

- Worker $w_2$ is not matched with his favorite $f_2$ in state 1. If not, $w_1$ is either single or matched with $f_3$ in state 1. Then, $w_1$ could deviate by moving $f_2$ just below $f_1$.

  Hence, $w_2$ must be matched with his second-best $f_3$ in all states.

  Finally, in state 1, $w_1$ and $w_3$ must be matched with $f_2$ and $f_1$, respectively, as desired.

In particular, in the corresponding unique BNE outcome, worker $w_2$ gets an expected utility of 2—he is matched with firm $f_3$ in all states.

Consider now the previous economy *augmented* with one additional worker $w_4$:

$\lambda_1$

$U(1)$

| | | | |
|---|---|---|---|
| $2,5$ | $4,1$ | $\mathbf{3,2}$ | $1,5$ |
| $\mathbf{4,2}$ | $3,5$ | $2,5$ | $1,1$ |
| $3,1$ | $\mathbf{4,2}$ | $1,1$ | $2,2$ |

$U(2)$

| | | | |
|---|---|---|---|
| $3,5$ | $2,1$ | $1,2$ | $\mathbf{4,5}$ |
| $\mathbf{3,2}$ | $1,5$ | $2,5$ | $4,1$ |
| $4,1$ | $\mathbf{3,2}$ | $2,1$ | $1,2$ |

$U(3)$

| | | | |
|---|---|---|---|
| $2,5$ | $1,1$ | $4,2$ | $\mathbf{3,5}$ |
| $2,2$ | $1,5$ | $\mathbf{3,5}$ | $4,1$ |
| $\mathbf{3,1}$ | $1,2$ | $2,1$ | $4,2$ |

Every state has a unique stable matching highlighted in bold in the payoff matrices. In line with Theorem 2.25 from Roth and Sotomayor (1992), in each state, no original worker is better off in the augmented economy, when stable matchings (and thus stable equilibrium outcomes) are compared.

In what follows, we demonstrate an unstable equilibrium outcome in the augmented economy that is preferred by original worker $w_2$ to the unique (stable) equilibrium outcome in the original economy. This stands in contrast to the complete-information setting, in which adding a worker never benefits other workers.

To be formal, consider the following profile of workers' weakly undominated strategies:

- $w_1$ and $w_2$ report truthfully;
- $w_3$ drops $f_1$;
- $w_4$ permutes $f_2$ and $f_3$.

This profile generates matchings $\lambda(\theta)$, $\theta \in \{1, 2, 3\}$. In each state, each of these matchings is the unique stable matching with respect to the reported preferences.

The proposed profile constitutes an equilibrium:

- Worker $w_3$ gets his favorite $f_2$ in state 3. In state 2, he cannot be matched with any firm (by inspecting the firm-proposing DA algorithm in that state). In state 1, he cannot be matched with $f_2$ (otherwise, $f_2$ and $w_2$ would block) or $f_3$ (otherwise, $f_3$ and any unmatched worker in that state would block). In order to get $f_1$ in state 1, $w_3$ needs to report $f_1$ as acceptable. However, such a deviation precludes him from getting his most preferred $f_2$ in state 3. The corresponding utility from $f_2$ is sufficiently high, so that $w_3$ has no incentives to deviate.
- Worker $w_4$ cannot be matched with $f_1$ in state 1 (otherwise, $f_1$ and $w_1$ would block), and thus has no incentives to deviate.
- Other workers have no incentives to deviate from their truthful strategies since the induced matchings are unique for the reported preferences.

To conclude, in the corresponding unstable BNE outcome, worker $w_2$ gets an expected payoff of $(5 + 2 + 0)/3 = 7/3 > 2$—he is matched with firm $f_2$ in state 1 and firm $f_3$ in state 2. When this equilibrium is selected, he is better off in the economy with worker $w_4$ compared to the original economy without that worker. △

## B. Proofs

**Proposition 2.** *Restrict workers' strategy sets to dropping strategies and consider any economy $\mathcal{E}$ such that either (1) all markets in its support do not have preference cycles; or (2) the SPC* is satisfied. Then, it admits a unique BNE outcome corresponding to the unique (complete-information) stable outcome in each state.*

**Proof.** By replicating arguments from the proof of Proposition 1, it is straightforward to prove (2).[2] We therefore focus on (1) and assume all markets in the support of $\mathcal{E}$ do not have preference cycles.

Consider first any *two-state* economy with sequential top-top pairs $\{(f_{i|\theta}, w_{i|\theta})\}_{i\leq \min(m,n)}$ in state $\theta \in \{1,2\}$, now defined in accordance with the "no-cycle" condition (that, in turn, implies the "standard" SPC). Since these two sequences correspond to unique stable matchings in the respective states, it suffices to prove that all top-top pairs must be matched in any BNE.

We apply induction on $k \leq \min(m,n)$, where $k$ is the number of pairs $\{(f_{i|\theta}, w_{i|\theta})\}_{i\leq k}$ in the sequences above. The assertion holds for $k = 1$. Indeed, the proof of Lemma 1 is valid even when workers' strategy sets are restricted to dropping strategies. Therefore, top-top matches must be matched under any BNE. Suppose that the assertion holds for $k \geq 1$. By the symmetry with respect to states, it suffices to prove that $(f_{k+1|1}, w_{k+1|1})$ must be matched to each other in state 1 under any BNE.

Suppose, towards a contradiction, that $(f_{k+1|1}, w_{k+1|1})$ are not matched in state 1 under some equilibrium yielding matching $\lambda(\theta)$ in state $\theta \in \{1,2\}$. Then, both $f_{k+1|1}$ and $w_{k+1|1}$ get less desirable assignments in state 1 under $\lambda(1)$. Because $f_{k+1|1}$ reports truthfully and workers employ dropping strategies, it follows that worker $w_{k+1|1}$ reports $f_{k+1|1}$ as unacceptable in his equilibrium (dropping) strategy $Q$. To reach a contradiction, it suffices to find him a

[2] Indeed, the deviations utilized in the proof of Proposition 1 are all dropping strategies.

profitable deviation.

Construct the candidate deviation $Q'$ from $Q$ by reporting $f_{k+1|1}$ as acceptable and adding her to $Q$ at her "true" place. That is, $Q'$ itself is also a dropping strategy, as required. Let $\lambda'(\theta)$ be a resulting stable matching in state $\theta \in \{1, 2\}$ for the reported preferences.

This proposed deviation strictly benefits $w_{k+1|1}$ in state 1. Suppose, towards a contradiction, that reporting $Q'$ instead of $Q$ hurts worker $w_{k+1|1}$ in state 2, so that $\lambda(2)(w_{k+1|1}) \succ_{w_{k+1|1}} \lambda'(2)(w_{k+1|1})$ with respect to his true preferences, and hence $Q'$. Then, there exists a cycle in preferences $(Q', Q_{rest})$, where $Q_{rest}$ is the profile of other agents' equilibrium preferences including firms' truthful rankings in state 2. This cycle allows worker $w_{k+1|1}$ to trigger a profitable rejection chain in state 2 by rejecting $f_{k+1|1}$. However, since all strategies in $(Q', Q_{rest})$ are dropping strategies, there must exist a cycle in truthful preferences as well, contradicting our assumption. Therefore, we must have $\lambda'(2)(w_{k+1|1}) \succeq_{w_{k+1|1}} \lambda(2)(w_{k+1|1})$, as desired.

Finally, for economies with more than two states, an identical proof works. Indeed, the same deviation is strictly beneficial in state 1 and weakly beneficial in any state $\theta \neq 1$. ∎

**Proposition 3.** *Consider any balanced market $\mathcal{M}$ with at least two agents on each side satisfying the SPC. Then, we can construct an augmented economy $\mathcal{E}$ of $\mathcal{M}$ with one additional firm and one additional worker such that:*

1. *there is a BNE that supports unstable outcomes in both states;*

2. *any BNE outcome can be supported by weakly undominated strategies that induce a unique stable matching (with respect to reported preferences) in each state;*

3. *the set of matched workers varies across equilibrium outcomes. Furthermore, workers disagree on which is preferred.*

**Proof.** Consider any market $\mathcal{M}$ satisfying the SPC for $\{f_i, w_i\}_{i\in[n]}$ (up to relabeling) and fix any non-degenerate binary distribution $\Psi$. To construct the desired augmented economy

$\mathcal{E}$, satisfying the three properties in the proposition, we add firm $f$ and worker $w$, so that

1. in both states, all firms $f_i$, $i \leq n-2$, rank the new worker $w$ as least desirable;
2. all workers $w_i$, $i \leq n-2$, rank the new firm $f$ as least desirable;
3. in both states, the new firm $f$ ranks all workers $w_i$, $i \leq n-2$, less desirable (in an arbitrary order) than $\{w_{n-1}, w_n, w\}$;
4. the new worker $w$ ranks all firms $f_i$, $i \leq n-2$, as less desirable than $\{f_{n-1}, f_n, f\}$;
5. all remaining preferences will be specified later to guarantee that stable matchings are unique in both states.

For this economy, for any stated preferences of workers $\{w_{n-1}, w_n, w\}$, all pairs $(f_i, w_i)$, $i \leq n-2$, are sequential top-top matches in both states, so they must be matched not only in any stable matching, but also in any BNE (not necessarily in weakly undominated strategies) by applying Lemma 1 repeatedly.

As a result, the new sub-economy formed by firms $\{f_{n-1}, f_n, f\}$ and workers $\{w_{n-1}, w_n, w\}$ can be considered "in isolation." In other words, it is sufficient to prove all results for the "bottom" two-by-two sub-market formed by $\{f_{n-1}, f_n\}$ and $\{w_{n-1}, w_n\}$.

By the SPC, worker $w_{n-1}$ must prefer $f_{n-1}$ to $f_n$ and firm $f_{n-1}$ must prefer $w_{n-1}$ to $w_n$, so that there are only four cases of preferences for the remaining worker $w_n$ and firm $f_n$:

1. $w_n$ prefers $f_{n-1}$ over $f_n$:
   (a) $f_n$ prefers $w_n$ over $w_{n-1}$;
   (b) $f_n$ prefers $w_{n-1}$ over $w_n$;
2. $w_n$ prefers $f_n$ over $f_{n-1}$:
   (a) $f_n$ prefers $w_n$ over $w_{n-1}$;

(b) $f_n$ prefers $w_{n-1}$ over $w_n$.

To conclude the proof, consider the following economies, where states $\Theta = \{1, 2\}$ are distributed according to the given $\Psi$ and $\rho \equiv \min(\Psi(1), 1 - \Psi(1)) \in (0, 1)$:

1. Example 1 above with

$U(1)$

| | | |
|---|---|---|
| $3, 2$ | $1, 2.5/\rho$ | $2, 2$ |
| $2, 2.5/\rho$ | $3, 2$ | $1, 2.5/\rho$ |
| $1, 1$ | $2, 1$ | $3, 1$ |

$U(2)$

| | | |
|---|---|---|
| $3, 2$ | $1, 2.5/\rho$ | $2, 2$ |
| $1, 2.5/\rho$ | $3, 2$ | $2, 2.5/\rho$ |
| $1, 1$ | $2, 1$ | $3, 1$ |

2. Example 2 above with

$U(1)$

| | | |
|---|---|---|
| $3, 2$ | $2, 2.5/\rho$ | $1, 1$ |
| $1, 1$ | $3, 2$ | $2, 2$ |
| $2, 2.5/\rho$ | $3, 1$ | $1, 2.5/\rho$ |

$U(2)$

| | | |
|---|---|---|
| $3, 2$ | $2, 2.5/\rho$ | $1, 1$ |
| $1, 1$ | $3, 2$ | $2, 2$ |
| $1, 2.5/\rho$ | $3, 1$ | $2, 2.5/\rho$ |

For each of the four cases, we can embed ordinal preferences for firms $\{f_{n-1}, f_n\}$ and workers $\{w_{n-1}, w_n\}$ into either of these two examples:

(1a) 1: $w_n$ = worker 3, $w_{n-1}$ = worker 1, $f_n$ = firm 3, and $f_{n-1}$ = firm 1;

(1b) 1: $w_n$ = worker 2, $w_{n-1}$ = worker 3, $f_n$ = firm 3, and $f_{n-1}$ = firm 1;

(2a) 2: $w_n$ = worker 3, $w_{n-1}$ = worker 1, $f_n$ = firm 2, and $f_{n-1}$ = firm 1;

(2b) 2: $w_n$ = worker 3, $w_{n-1}$ = worker 2, $f_n$ = firm 2, and $f_{n-1}$ = firm 1.

Although the original utilities for $\{w_{n-1}, w_n, f_{n-1}, f_n\}$ are fixed and may be different from the ones in the examples, we can apply an appropriate positive affine transformation for the

utilities of workers $\{w_{n-1}, w_n\}$. It is feasible since, for each worker, we need to map only two utilities for $f_{n-1}$ and $f_n$, and any monotone transformation for firms $\{f_{n-1}, f_n\}$—firms report their truthful preferences, so that only ordinal firms' preferences matter.

Finally, as shown above, all statements of the proposition hold for both examples and, hence, for our constructed economy. ∎

## C. Generalization of Stability Results

In this section, we show that Propositions 1 and 2 of Section 4 in the paper continue to hold for a *generalized centralized matching economy* game that, among other things, allows for two-sided incomplete information and type-dependent beliefs.

As in the main text, we consider a finite set of states $\Theta$, where each state $\theta$ is associated with utilities $U(\theta) = (u^f_{1\cdot}(\theta), \ldots, u^f_{m\cdot}(\theta), u^w_{\cdot 1}(\theta), \ldots, u^w_{\cdot n}(\theta))$ for firms $F = \{f_i\}_{i \in [m]}$, and workers $W = \{w_j\}_{j \in [n]}$. In what follows, we relax the common prior assumption.

For each firm $f_i$, we describe her information by a *partition* $\Pi^f_i$ of $\Theta$. For any state $\theta \in \Theta$, we write $\Pi^f_i(\theta)$ for the partition cell $\Pi^f_i$ containing $\theta$. When the true state is $\theta$, firm $f_i$ regards each state in $\Pi^f_i(\theta)$ as possible. Firm $f_i$'s "type" is given by her partition cell. We suppose that for every state $\theta \in \Theta$, we have $\Pi^f_i(\theta) \subseteq \{\theta' \in \Theta : u^f_{i\cdot}(\theta) = u^f_{i\cdot}(\theta')\}$. Informally, each firm distinguishes between states with different utility functions and possibly between some states with identical utility functions. In addition, each firm $f_i$ is endowed with her type-dependent beliefs given by a function $\Phi^f_i$ that maps every partition cell $\Pi^f_i(\theta)$—her type—to some probability distribution with support $\Pi^f_i(\theta)$. For each worker $w_j$, we make analogous assumptions and define his partition $\Pi^w_j$ and type-dependent beliefs $\Phi^w_j$ accordingly.

*Remark* 1. Our setup with one-sided incomplete information from the main paper corresponds to: (1) uninformed workers with state-independent utilities, so that $\Pi^w_j = \{\Theta\}$ and $\Phi^w_j(\Theta) = \Psi$ for all $j$, where $\Psi$ is a common prior; (2) informed firms with possibly state-

dependent utilities, so that $\Pi_i^f = \{\{\theta\}\}_{\theta\in\Theta}$ and degenerate $\Phi_i^f(\{\theta\})$ placing all probability on $\theta$ for all $i$ and $\theta$.

*Remark* 2. The classic setting from Roth (1989) naturally fits into our setup. Specifically, he assumes that each firm $f_i$'s type is given by her utility function from a finite set $U_i^f$ of utility functions. Similarly, each worker $w_j$'s type is given by his utility function from a finite set $U_j^w$. Let $G$ denote the joint distribution over agents' utility profiles $U \equiv \prod_i U_i^f \times \prod_j U_j^w$. At the time in which (Bayesian) agents choose their strategies, each agent knows her own type and the probability distribution $G$. In particular, each agent's utility payoff depends on his own type and on other players' actions, but not on other players' types.

We can translate Roth's setting to our setup by taking the state space $\Theta = \operatorname{supp} G$, partitions $\Pi_i^f(u) = \{u' \in \Theta : u'^f_{i\cdot} = u^f_{i\cdot}\}$ and $\Pi_j^w(u) = \{u' \in \Theta : u'^w_{\cdot j} = u^w_{\cdot j}\}$, and beliefs $\Phi_i^f$ and $\Phi_j^w$ induced by $G$.

A *centralized matching mechanism* $\varphi$ is a function that inputs reports of preferences from all agents and outputs a matching. In what follows, we assume that a matching mechanism asks each agent to report her ranking only over her set of acceptable partners (if any). A mechanism is *stable* if it selects a stable matching for each profile of reported preferences. In particular, let $\varphi^F$ be the firm-proposing DA mechanism analyzed in the paper.

Consider the direct-revelation game $\Gamma(\varphi^F)$ induced by the firm-proposing DA mechanism with two-sided incomplete information specified above. A *strategy* for agent $a \in F \cup W$ is a function mapping every partition cell ($a$'s type) to a reported ranking of acceptable partners. A *truth-telling* strategy reports, for every partition cell, the corresponding true ranking.

Under (in)complete information, the firm-proposing DA makes it weakly dominant for firms to report truthfully. This is due to strategy-proofness of the DA for the proposing agents (Dubins and Freedman, 1981; Roth, 1982) and the result below.

**Claim 1.** *Consider any stable mechanism $\varphi$ and any agent $a \in F \cup W$. Then, for any ranking $\succ'_a \neq \succ_a$, there exist rankings $\succ_{-a}$ for other agents such that $\varphi(\succ_a, \succ_{-a}) \succ_a \varphi(\succ'_a, \succ_{-a})$.*

**Proof.** Without loss of generality, consider any $a = f \in F$ with arbitrary rankings $\succ'_f \neq \succ_f$. There are three cases to consider:

1. If $w$ is acceptable under $\succ'_f$, but not $\succ_f$, consider $\succ_{-f}$ in which $w$ reports $f$ as the only acceptable firm and other agents have no acceptable partners.

2. If $w$ is acceptable under $\succ_f$, but not $\succ'_f$, consider the same $\succ_{-f}$ as above.

3. Suppose $\succ_f$ and $\succ'_f$ specify the same set of acceptable workers including $w$ and $w' \neq w$, but $f$ prefers $w$ to $w'$ under $\succ_f$ and $w'$ to $w$ under $\succ'_f$. Then, consider $\succ_{-f}$ in which both $w$ and $w'$ report $f$ as the only acceptable firm and other agents have no acceptable partners. ∎

We then have:

**Claim 2.** *Truth-telling is (interim) weakly dominant for firms in the game $\Gamma(\varphi^F)$ with two-sided incomplete information. If, in addition, firm $f_i$ is Bayesian with a full-support prior, truth-telling is also ex-ante weakly dominant for her.*[3]

**Proof.** Since $\varphi^F$ is strategy-proof for firms, both types of weak dominance follow trivially from Claim 1. Indeed, suppose a firm $f$ reports untrue $\succ'_f$ instead of her true $\succ_f$ for some partition cell (type). We can consider all other agents employing constant strategies coinciding with $\succ_{-f}$ constructed in Claim 1. ∎

[3] In games with incomplete information there are two notions of dominance: ex-ante dominance and interim dominance (see, e.g., pages 226-229 in Fudenberg and Tirole, 1991). Ex-ante dominance requires that all types of an agent have the same beliefs about the play of the other players. In contrast, interim dominance allows different types to have different beliefs.

Therefore, we restrict attention to Bayesian Nash equilibria (BNE) in which firms report their preferences truthfully, as in the main paper.[4]

The SPC condition is defined as in the main text with only one difference—now, workers may have state-dependent utilities. The SPC* condition is generalized as follows.

**Definition 1.** *An economy $\mathcal{E}$ satisfies the SPC* if it satisfies the SPC and, for any state $\theta \in \Theta$, and any order $i \leq \min(m, n)$,*

$$\text{if } f \succ_{w_{i|\theta}} f_{i|\theta}, \text{ then for any } \theta' \in \Pi_i^w(\theta), \text{ there exists } i' < i \text{ (that may depend on } \theta'\text{) with } f = f_{i'|\theta'},$$

*where $\succ_{w_{i|\theta}}$ is $w_{i|\theta}$'s preference in state $\theta$, and hence corresponding to partition cell $\Pi_i^w(\theta)$.*

That is, if in some state $\theta \in \Theta$, a worker of a given order prefers some firm over her stable partner in this state, then in any state $\theta' \in \Pi_i^w(\theta)$ that he cannot "distinguish" from the given one, this firm must have a smaller order.

With the generalized SPC* condition in hand, we can extend our original stability results. Below are proofs for Lemma 1 and Proposition 1 (appearing in Section 4 of the main text) for our general setup with two-sided incomplete information. For completeness, we include their statements, which replicate those in the paper.

**Lemma 1*.** *Consider any economy $\mathcal{E}$. If firm $f_i$ and worker $w_j$ form a top-top match pair in state $\theta$, they must be matched in this state under any BNE.*

**Proof.** Since firms employ truth-telling strategies, firm $f_i$ reports worker $w_j$ as her top choice for her partition cell $\Pi_i^f(\theta) \ni \theta$. If they are not matched in state $\theta$, then for his partition cell $\Pi_j^w(\theta) \ni \theta$, $w_j$'s top-ranked firm is not his true first choice $f_i$. Therefore, $w_j$ could profitably deviate by shifting $f_i$ to the top of his ranking corresponding to $\Pi_j^w(\theta)$ to strictly benefit in state $\theta$ without losing in other states $\theta' \in \Pi_j^w(\theta)$, $\theta' \neq \theta$. ∎

[4] Formally, a *Bayesian Nash equilibrium* is a strategy profile that for each type of each agent, maximizes her expected payoff, given other agents' strategies (see page 215 in Fudenberg and Tirole, 1991).

**Proposition 4*.** *Consider any economy $\mathcal{E}$ such that either (1) firms have (possibly state-specific) assortative preferences or (2) the SPC* is satisfied. Then, it admits a unique BNE outcome corresponding to the unique (complete-information) stable outcome in each state.*

**Proof.** Consider any economy with sequential top-top pairs $\{(f_{i|\theta}, w_{i|\theta})\}_{i\leq \min(m,n)}$ in state $\theta \in \Theta$, defined in accordance with firms' assortative preferences (that, in turn, imply the "standard" SPC) for part (1) or the SPC* condition for part (2). Since these top-top pair sequences correspond to unique stable matchings in the respective states, it is sufficient to prove that all top-top pairs must be matched under any BNE.

We apply induction on $k \leq \min(m,n)$, where $k$ is the number of the first pairs $\{(f_{i|\theta}, w_{i|\theta})\}_{i\leq k}$ in the sequences above. The assertion holds for $k = 1$. Indeed, by Lemma 1*, top-top matches must be matched under any BNE. Suppose that the assertion holds for $k \geq 1$. By symmetry with respect to states, it suffices to prove that $(f_{k+1|1}, w_{k+1|1})$ must be matched to each other in state 1 under any BNE.

Suppose, towards a contradiction, that $(f_{k+1|1}, w_{k+1|1})$ are not matched in state 1 under some equilibrium yielding matching $\lambda(\theta)$ in state $\theta \in \Theta$. Then, both $f_{k+1|1}$ and $w_{k+1|1}$ get less desirable assignments in state 1 under $\lambda(1)$. Because $f_{k+1|1}$ uses her truth-telling strategy, this implies that worker $w_{k+1|1}$, for his partition cell $\Pi^w_{k+1|1}(1) \ni 1$, reports the less desirable $\lambda(1)(w_{k+1|1})$ as preferable to $f_{k+1|1}$ in his equilibrium strategy.

As in the original proof, worker $w_{k+1|1}$ could profitably deviate by changing his ranking corresponding to $\Pi^w_{k+1|1}(1)$ to strictly benefit in state 1 without losing in other states $\theta \in \Pi^w_{k+1|1}(1)$, $\theta \neq 1$. Indeed, for part (1), $w_{k+1|1}$ could deviate by using his truthful ranking corresponding to $\Pi^w_{k+1|1}(1)$. As concerns part (2), $w_{k+1|1}$ could deviate by shifting firms $\{f : f \succeq_{w_{k+1|1}} f_{k+1|1}\}$, ranked truthfully, to the top of his equilibrium ranking corresponding to $\Pi^w_j(\theta)$, where $\succ_{w_{k+1|1}}$ above denotes $w_{k+1|1}$'s true preference in state 1, and hence corresponding to partition cell $\Pi^w_{k+1|1}(1)$. ∎

In a similar way, we can generalize Proposition 2 stated in the paper. Its formulation and proof are omitted for brevity.

## D. Fragility of General Stable Mechanisms

In this section, we show that a large class of stable mechanisms including quantile stable mechanisms (formally defined below) might have unstable equilibrium outcomes under incomplete information.

**D.1. Preliminaries.** Before proving our fragility result, we state the following dominance principle that we use in both the main paper and this section to construct (interim) weakly undominated strategies.

**Claim 3.** *Consider any matching mechanism $\varphi$ and the induced direct-revelation game $\Gamma(\varphi)$ with two-sided incomplete information specified above. Then, any agent's strategy employing a complete-information weakly undominated strategy for each partition cell is itself (interim) weakly undominated.*

**Proof.** This follows directly since we can always consider all other agents employing constant strategies. ∎

When combined with Claim 3, Claim 1 implies that for any stable mechanism $\varphi$, truth-telling is (interim) weakly undominated in the induced game $\Gamma(\varphi)$.

In addition, in our analysis, we also rely on the following result to construct (interim) weakly undominated strategies for workers in the induced game $\Gamma(\varphi)$ for a class of stable mechanisms $\varphi$ that agree with $\varphi^F$ for each profile with two stable matchings.

**Claim 4.** *Consider any stable mechanism $\varphi$ that agrees with $\varphi^F$ for each profile with two stable matchings. Suppose that $|W| \geq 2$ and let $\succ'_w$ be any ranking for $w \in W$ in which*

*(a)* $f_1 \in F$ *(w's true first choice) is listed first, and (b) the acceptable firms in* $\succ'_w$ *are also acceptable in w's true ranking* $\succ_w$*. Then, for any other ranking* $\succ''_w \neq \succ'_w$ *there exist rankings* $\succ_{-w}$ *for the other players such that* $\varphi(\succ'_w, \succ_{-w}) \succ_w \varphi(\succ''_w, \succ_{-w})$*.*[5]

**Proof.** Consider any $w \in W$ with any preferences $\succ_w$ and arbitrary rankings $\succ''_w \neq \succ'_w$.

Assume first that $f_1$ is not $\succ''_w$'s reported first choice. Then, consider $\succ_{-w}$ in which all firms report $w$ as the only acceptable worker and other agents have no acceptable partners.

In the remainder of the proof, we restrict attention to rankings $\succ''_w$ that list $f_1$ at the top. There are three relevant cases.

1. If $f$ is acceptable under $\succ'_w$, but not $\succ''_w$, consider $\succ_{-w}$ in which $f$ reports $w$ as the only acceptable worker and other agents have no acceptable partners.

2. If $f \neq f_1$ is acceptable under $\succ''_w$, but not $\succ'_w$, consider $\succ_{-w}$ in which

$$f : w \succ w' \qquad\qquad w' : f \succ f_1$$
$$f_1 : w' \succ w$$

   for some $w' \neq w$, $w' \in W$, and other agents have no acceptable partners. Then, $\varphi$ agrees with $\varphi^F$ on both $(\succ''_w, \succ_{-w})$ and $(\succ'_w, \succ_{-w})$ that admit at most two stable matchings. Furthermore, $w$ gets his favorite $f_1$ under $\succ'_w$, but only $f$ under $\succ''_w$.

3. Let $\succ'_w$ and $\succ''_w$ contain the same set of acceptable firms including $f \neq f_1$ and $f' \neq f, f_1$,

[5] This claim generalizes Theorem 6 from Gale and Sotomayor (1985) beyond the firm-proposing DA mechanism $\varphi^F$. Its proof is almost identical to the one of Theorem 6. For the sake of completeness, we provide the complete proof here.

but $w$ prefers $f$ to $f'$ under $\succ'_w$ and $f'$ to $f$ under $\succ''_f$. Then, consider $\succ_{-w}$ in which

$$f : w \succ w' \qquad\qquad w' : f' \succ f_1 \succ f$$
$$f' : w \succ w'$$
$$f_1 : w' \succ w$$

for some $w' \neq w$, $w' \in W$, and other agents have no acceptable partners. As before, $\varphi$ agrees with $\varphi^F$ on both $(\succ''_w, \succ_{-w})$ and $(\succ'_w, \succ_{-w})$ that admit at most two stable matchings. It is straightforward to check that $w$ gets his favorite $f_1$ under $\succ'_w$, but only $f'$ under $\succ''_w$. ∎

*Remark* 3. In particular, Claim 4 holds for so-called *quantile stable mechanisms.* These mechanisms generate stable matchings that can be seen as a compromise between the two market sides.

Formally, for any $q \in [0, 1]$, the *q-quantile stable mechanism* $\varphi^q$ assigns each firm her $\max(\lceil kq \rceil, 1)$-th best outcome among all matchings that are stable under the reported preferences, where $k$ is the number of such stable matchings.[6] Quantile stable mechanisms are well-defined stable mechanisms (see Chen et al., 2016, 2021 and references therein). The firm-proposing and worker-proposing DA are special cases—$\varphi^0 = \varphi^F$, $\varphi^1 = \varphi^W$—as is the median stable mechanism $\varphi^{1/2}$.[7]

It is easy to see that for any $q \in [0, 1/2]$, $\varphi^q$ agrees with $\varphi^F$ for each profile with two stable matchings, and thus is covered by the previous claim.

To conclude this subsection, note that for our setting with everyone being acceptable, Claims 3 and 4 imply that any worker strategy that, for each partition cell, lists the corre-

[6] $\lceil x \rceil$ denotes the lowest integer equal to or larger than $x$. We use the maximum operator for $\varphi^q$ to be well-defined for $q = 0$.

[7] Echenique and Yariv (2013) in their experiments show that in decentralized two-sided matching markets with multiple stable matchings, agents tend to coordinate on the median stable matching.

sponding most-preferred firm first is (interim) weakly undominated in any $\Gamma(\varphi)$ induced by a stable mechanism $\varphi$ that agrees with $\varphi^F$ on each profile with two stable matchings.

**D.2. Fragility Results.** The following modification of our motivating example will be useful in illustrating our general fragility result.

$\lambda$

$U(1)$

| | | |
|---|---|---|
| **3, 2** | 1, 5 | 2, 2 |
| 2, 5 | **3, 2** | 1, 5 |
| 3, 1 | 1, 1 | **2, 1** |

$U(2)$

| | | |
|---|---|---|
| **3, 2** | 1, 5 | 2, 2 |
| 1, 5 | **3, 2** | 2, 5 |
| 1, 1 | 2, 1 | **3, 1** |

Consider an economy with three firms, three workers, and two equally likely states. As in the motivating example, there is no uncertainty regarding the stable matching $\mu$, $\mu(f_i) = w_i$ for $i \in \{1, 2, 3\}$, highlighted in bold.

Furthermore, suppose $\varphi$ is any stable mechanism that agrees with the firm-proposing DA mechanism $\varphi^F$ for each profile with two stable matchings. It is no longer weakly dominant for firms to report truthfully. In what follows, we analyze BNE in interim weakly undominated strategies for all agents (where agents can "use" any information at their disposal).

Consider the following profile of strategies for all agents:

- all firms and $w_3$ report truthfully;
- $w_1$ reports only $f_2$ as acceptable;
- $w_2$ permutes $f_2$ and $f_3$.

It generates unique stable matchings for the reported preferences, $\lambda(1)$ and $\lambda(2)$ in states 1 (left) and 2 (right), that are selected by any stable mechanism including $\varphi$.

By our analysis in the previous subsection, all stated strategies are interim weakly undominated. Indeed, for each truthful agent, we can use Claims 1 and 3. Similarly, for workers $w_1$ and $w_2$, we can apply Claims 3 and 4.

In fact, they constitute an equilibrium:

- All firms and $w_3$ have no incentives to deviate from truth-telling since the induced matchings are unique for reported preferences and $\varphi$ is stable.

- Worker $w_1$ gets his favorite $f_2$ in state 1 and cannot get her in state 2 (otherwise, $f_2$ and $w_3$ would block in state 2). Then, to deviate profitably, $w_1$ needs to keep $f_2$ in state 1 and get either $f_1$ of $f_3$ in state 2. Below, we show that $w_1$ has no profitable deviations.

  Note first that $w_1$ needs to report $f_2$ as acceptable and rank her above both $f_1$ and $f_2$ (otherwise, he would not be matched with $f_2$ in state 1). Therefore, we need to check four strategies:

$$f_2 \succ f_1 \succ f_3$$
$$f_2 \succ f_3 \succ f_1$$
$$f_2 \succ f_1$$
$$f_2 \succ f_3$$

  Second, it is straightforward to check that for all deviations above, there are two stable matchings in state 1, so that (a) $\lambda(1)$ is the worker-optimal stable one in all four cases, and (b) $w_1$ is matched with either $f_1$ or $f_3$ in the firm-optimal stable matching. Finally, since $\varphi$ agrees with the firm-proposing DA mechanism $\varphi^F$ for each profile with two stable matchings, $w_1$ cannot keep his favorite $f_2$ in state 1 for each deviation, and thus they are not profitable.

- Similarly, worker $w_2$ gets his favorite $f_1$ in state 2 and cannot get her in state 1 (otherwise, $f_1$ and $w_3$—who himself cannot be matched with $f_2$ in state 1—would block in state 1). Therefore, to deviate profitably, $w_2$ needs to keep $f_1$ in state 2 and get his second-best $f_2$ in state 1.

  Note that we can use the firm-proposing DA mechanism $\varphi^F$ instead of $\varphi$ to analyze $w_2$'s deviations. Indeed, since $w_1$ reports only $f_2$ as acceptable, we can have at most two stable matchings in each state.

  Under the firm-proposing DA mechanism $\varphi^F$, in order to get $f_2$ in state 1, $w_2$ needs to report $f_2$ as preferable to $f_3$. However, such a deviation precludes him from getting his most preferred $f_1$ in state 2. Therefore, it is not profitable.

Based on our analysis so far, we can state the following fragility result. Note that

**Proposition 5.** *There exists an economy with a profile of strategies that constitutes a BNE in interim undominated strategies with unstable outcomes in all states for any stable mechanism $\varphi$ that agrees with the firm-proposing DA mechanism $\varphi^F$ for each profile with two stable matchings. In particular, it holds for any q-quantile stable mechanism $\varphi^q$ with $q \in [0, 1/2]$.*

For conciseness, we omit additional features of the constructed economy and the respective equilibrium profile. In particular, firms uniformly prefer the corresponding equilibrium to the stable one and the set of matched workers varies across equilibrium outcomes.[8]Also, the constructed profile induces a unique stable matching in each state.

Why do we modify our motivating example to obtain the result above? As it turns out, all profiles corresponding to $\lambda_1$ or $\lambda_2$ (see Example 1 from Appendix A) do not constitute an equilibrium even for the median stable mechanism $\varphi^{1/2}$.All profiles corresponding to $\lambda_3$

[8]Note that for any stable mechanism, ex-post stable outcomes are always implemented by all agents reporting truthfully.

continue to be an equilibrium for $\varphi^q$ with $q \in [0, 1/2]$, but may fail to do so for more general classes of mechanisms we consider above.

Certainly we can "tranpose" the example above by changing the roles of firms and workers to establish an analogous result for any stable mechanism $\varphi$ that agrees with the worker-proposing DA mechanism $\varphi^W$ for each profile with two stable matchings, and particularly for any $q$-quantile stable mechanism $\varphi^q$ with $q \in (1/2, 1]$. Based on this observation, we can combine the example above with its "transpose"—say, by keeping the same agents, but adding two extra states—to obtain the following.

**Corollary 1.** There exists an economy such that for any mechanism $\varphi$ that agrees with either (1) the firm-proposing DA mechanism $\varphi^F$ for each profile with two stable matchings, or (2) the worker-proposing DA mechanism $\varphi^W$ for each such profile, there is a BNE in interim undominated strategies with unstable outcomes in some states.In particular, it holds for any $q$-quantile stable mechanism $\varphi^q$, $q \in [0, 1]$

Corollary 1 covers common classes of stable mechanisms used in practice. Nevertheless, what can we say about stable mechanisms not covered by our analysis?

In fact, in contrast to the DA mechanisms, arbitrary stable mechanisms might have equilibria in weakly undominated strategies with unstable outcomes even under complete information. The example below illustrates that all stable mechanisms that are different from the DA mechanisms for markets with two workers and two firms might have such an unstable equilibrium even for a fully assortative market.[9]

**Example 10.** For markets with two agents on either side, we have only two profiles of strategies with multiple stable matchings:

[9] The example below is based on Example 9 in Ma (1995).

$$f_1 : w_2 \succ w_1 \qquad\qquad w_1 : f_1 \succ f_2$$

$$f_2 : w_1 \succ w_2 \qquad\qquad w_2 : f_2 \succ f_1$$

and

$$f_1 : w_1 \succ w_2 \qquad\qquad w_1 : f_2 \succ f_1$$

$$f_2 : w_2 \succ w_1 \qquad\qquad w_2 : f_1 \succ f_2$$

.

Therefore, when restricted to such markets, there are only two non-DA stable mechanisms. Without loss of generality, focus on the stable mechanism that chooses the worker-optimal stable matching for the former profile and the firm-optimal stable matching for the latter profile.

Consider the following fully assortative market

$$f_1 : w_1 \succ w_2 \qquad\qquad w_1 : f_1 \succ f_2$$

$$f_2 : w_1 \succ w_2 \qquad\qquad w_2 : f_1 \succ f_2$$

with the unique stable matching $\mu(f_i) = w_i$, $i = 1, 2$.

Then, the profile of strategies

$$f_1 : w_1 \succ w_2 \qquad\qquad w_1 : f_1 \succ f_2$$

$$f_2 : w_1 \qquad\qquad w_2 : f_1$$

constitutes a NE in weakly undominated strategies and generates the unstable matching $\lambda(f_1) = w_1$, $\lambda(f_2) = f_2$, $\lambda(w_2) = w_2$.

Indeed, $f_1$ and $w_1$ have no incentives to deviate, $f_2$ cannot do better by unilaterally listing $w_2$, and $w_2$ cannot do better by unilaterally listing $f_2$.

As for the employed strategies, by Claim 1, truthful-telling is weakly undominated for $f_1$ and $w_1$. Furthermore, truncation is weakly undominated for $f_2$: it is the unique best response

for the first profile with two stable matchings. Similarly, truncation is undominated for $w_2$: it is the unique best response for the second profile with two stable matchings.[10,11] △

Thus, under complete information and the concept of weakly undominated NE, stable mechanisms other than the DA mechanisms might be prone to coordination issues—acceptable partners might declare one another unacceptable, which is robust to unilateral deviations.

To conclude, the general analysis of arbitrary stable mechanisms is also complicated by the absence of results regarding weakly undominated strategies even for the complete-information setting.[12]

## References


**Alcalde, Jose**, "Implementation of Stable Solutions to Marriage Problems," *Journal of Economic Theory*, 1996, *69* (1), 240–254.

**Chen, Peter, Michael Egesdal, Marek Pycia, and M. Bumin Yenmez**, "Median Stable Matchings in Two-Sided Markets," *Games and Economic Behavior*, 2016, *97*, 64–69.

**_ , _ , _ , and _** , "Quantile Stable Mechanisms," *Games*, 2021, *12* (2), 43.

**Dubins, Lester E. and David A. Freedman**, "Machiavelli and the Gale-Shapley Algorithm," *The American Mathematical Monthly*, 1981, *88* (7), 485–494.

**Echenique, Federico and Leeat Yariv**, "An Experimental Study of Decentralized Matching," 2013.


[10]Note that we cannot use Claim 4 directly.

[11]This example also shows that Proposition 1 cannot be generalized to arbitrary stable mechanisms even for complete-information fully assortative markets and the concept of undominated NE.

[12]Without requiring weakly undominated strategies, any stable mechanism, including the DA, is known to implement the set of individually rational matchings under complete information (e.g., see Alcalde, 1996).

**Ferdowsian, Andrew, Muriel Niederle, and Leeat Yariv**, "Decentralized Matching with Aligned Preferences," 2021.

**Fudenberg, Drew and Jean Tirole**, *Game theory*, MIT press, 1991.

**Gale, David and Marilda Sotomayor**, "Ms. Machiavelli and the Stable Matching Problem," *The American Mathematical Monthly*, 1985, *92* (4), 261–268.

**Ma, Jinpeng**, "Stable Matchings and Rematching-Proof Equilibria in a Two-Sided Matching Market," *Journal of Economic Theory*, 1995, *66* (2), 352–369.

**Roth, Alvin E.**, "The Economics of Matching: Stability and Incentives," *Mathematics of Operations Research*, 1982, *7* (4), 617–628.

_ , "Two-Sided Matching with Incomplete Information about Others' Preferences," *Games and Economic Behavior*, June 1989, *1* (2), 191–209.

_ **and Marilda A. Oliveira Sotomayor**, *Two-Sided Matching: A Study in Game-Theoretic Modeling and Analysis* Econometric Society Monographs, Cambridge: Cambridge University Press, 1992.
